# Supplementary material for: High-Performance Large-Scale Image Recognition Without Normalization
Source: arXiv:2102.06171 source file (2021-02-11)
Supplement: Supplementary file 1 [file Appendix_AGC_Code.tex]

\begin{minted}{python}
"""Adaptive gradient clipping transform for Optax."""
import jax
import jax.numpy as jnp
import optax


def mynorm(x, axis, keepdims):
  """Axis-wise euclidean norm."""
  return jnp.sum(x ** 2, axis=axis, keepdims=keepdims) ** 0.5


def unitwise_norm(x):
  """Compute norms of each output unit separately, also for linear layers."""
  if len(jnp.squeeze(x).shape) <= 1:  # Scalars and vectors
    axis = None
    keepdims = False
  elif len(x.shape) in [2, 3]:  # Linear layers of shape IO or multihead linear
    axis = 0
    keepdims = True
  elif len(x.shape) == 4:  # Conv kernels of shape HWIO
    axis = [0, 1, 2,]
    keepdims = True
  else:
    raise ValueError(f'Got a parameter with shape not in [1, 2, 4]! {x}')
  return mynorm(x, axis, keepdims)


def my_clip(g_norm, max_norm, grad):
  """Applies my gradient clipping unit-wise."""
  trigger = g_norm < max_norm
  # This little max(., 1e-6) is distinct from the normal eps and just prevents
  # division by zero. It technically should be impossible to engage.
  clipped_grad = grad * (max_norm / jnp.maximum(g_norm, 1e-6))
  return jnp.where(trigger, grad, clipped_grad)


def adaptive_grad_clip(clip, eps=1e-3) -> optax.GradientTransformation:
  """Clip updates to be at most clipping * parameter_norm.

 
  Args:
    clip: Maximum allowed ratio of update norm to parameter norm.
    eps: epsilon term to prevent clipping of zero-initialized params.

  Returns:
    An (init_fn, update_fn) tuple.
  """

  def init_fn(_):
    return optax.ClipByGlobalNormState()

  def update_fn(updates, state, params):
    g_norm = jax.tree_map(unitwise_norm, updates)
    p_norm = jax.tree_map(unitwise_norm, params)
    # Maximum allowable norm
    max_norm = jax.tree_map(lambda x: clip * jnp.maximum(x, eps), p_norm)
    # If grad norm > clipping * param_norm, rescale
    updates = jax.tree_multimap(my_clip, g_norm, max_norm, updates)
    return updates, state

  return optax.GradientTransformation(init_fn, update_fn)

\end{minted}
