# Supplementary material for: High-Performance Large-Scale Image Recognition Without Normalization
Source: arXiv:2102.06171 source file (2021-02-11)
Supplement: Supplementary file 2 [file Appendix_NFResNetBlock_Ablations.tex]

\begin{table*}[htb]
\begin{center}
\begin{tabular}{l| l | c | c | c}
\toprule [0.15em]
                           & & BS 256 & BS 1024 & BS 4096 \\
\midrule [0.1em]
\multirow{7}{*}{ResNet50}  & Batch normalization & $76.7 \pm 0.1$ & $76.7 \pm 0.1$ & $76.9 \pm 0.1$ \\
                           & SkipInit & $76.0 \pm 0.1$ & $76.2 \pm 0.2$ & $72.2 \pm 0.3$ \\
                           & + Scaled WS & $76.8 \pm 0.1$ & $77.0 \pm 0.1$ & $76.0 \pm 0.1$ \\
                           & (1) + (2) & $76.9 \pm 0.1 ^\star$ & $77.1 \pm 0.1$ & $75.8 \pm 0.1$ \\
                           & (1) + (2) + (3) & $77.0 \pm 0.1$ & $77.1 \pm 0.0$ & $75.2 \pm 0.1$ \\
                           & (1) + (2) + (4) & $76.9 \pm 0.1$ & $77.0 \pm 0.1$ & $74.8 \pm 0.2 ^\star$ \\
                           & (1)+(2)+(3)+(4) (NF-ResNet) & $76.9 \pm 0.2$ & $77.0 \pm 0.1$ & $76.0 \pm 0.1$ \\
\midrule [0.1em]
\multirow{7}{*}{ResNet200}  & Batch normalization & $79.0 \pm 0.1$ & $79.1 \pm 0.1$ & $79.1 \pm 0.1$  \\
                           & SkipInit & $78.7 \pm 0.1$ & $78.8 \pm 0.1^\star$ & $72.7 \pm 0.2$ \\
                           & + Scaled WS & $79.5 \pm 0.1^\star$ & $79.7 \pm 0.1$ & $78.6 \pm 0.1$ \\
                           & (1) + (2) & --  & -- & -- \\
                           & (1) + (2) + (3) & $79.8 \pm 0.1^\star$ & $79.9 \pm 0.1^\star$ & $77.5 \pm 0.0^\star$ \\
                           & (1) + (2) + (4) & $79.2 \pm 0.1$ & $79.3 \pm 0.1 ^\star$ & $77.1 \pm 0.1$ \\
                           & (1)+(2)+(3)+(4) (NF-ResNet)  & $79.5 \pm 0.2$ & $79.6 \pm 0.1$ & $78.5 \pm 0.1$ \\
\bottomrule[0.15em]
\end{tabular}
\end{center}

\caption{\label{table:resnet_block_ablations} Ablation table on the NF-ResNet block compared to batch normalization and SkipInit. (1), (2), (3) and (4) denote the four modifications described in Section \ref{appendix:resnetblock_ablations}. $^\star$ indicates a setting which is unstable, where more than one independent run failed (results are averaged over successful runs in this case). -- indicates a setting where all runs failed.}
\end{table*}

\section{Ablations on the NF-ResNet Block Design}
\label{appendix:resnetblock_ablations}

In this paper, we build on Normalizer-Free ResNets (NF-ResNets) introduced by \citet{brock2021characterizing}. In this section, we present results of ablations that show the efficacy of the main ResNet block used in NF-ResNets.

After removing the batch normalization layers from pre-activation ResNets, NF-ResNets involve making the following modifications to the ResNet block:
\begin{enumerate}[label=(\arabic*)]
    \item The input to the $i^{th}$ residual branch is downscaled by a scalar $\beta_i$, where $\beta_i$ is determined by predicting the standard deviation of the inputs to the $i^{th}$ residual block: $\beta_i = \sqrt{\text{Var}(h_i)}$, where $h_i$ denotes the input to the $i^{th}$ residual block.
    \item Apply Scaled Weight Standardization on the convolutional layers, as defined in Equation \ref{eq:scaled_ws}. Additionally scale the activation function by the non-linearity specific scalar $\gamma$, which ensures that the combination of the $\gamma$-scaled activation function and a Scaled Weight Standardized layer is variance preserving.
    \item Multiply the output of each residual branch by a constant scalar $\alpha = 0.2$.
    \item Multiply the output of each residual branch by a learnable scalar multiplier initialized to zero.
\end{enumerate}

In Table \ref{table:resnet_block_ablations}, we present results of ablations to show the effect of making these four modifications to unnormalized ResNets across 3 different batch sizes. We compare these runs to batch normalized ResNets and SkipInit \citep{de2020batch} with and without Scaled Weight Standardization (Scaled WS). We use Dropout with drop rate 0.25 \citep{srivastava2014dropout} and Stochastic Depth with rate 0.1 \citep{huang2016deep} on models not using batch normalization to recover the implicit regularization effects of batch normalization \citep{hoffer2017train}. For each method and batch size, we tune the learning rate on a logarithmic grid. We perform 7 independent runs, and provide results for the optimal learning rate averaged over the runs that successfully trained. To indicate stability of each method, we use a $^\star$ to indicate settings where more than one independent run failed to train.

From Table \ref{table:resnet_block_ablations}, we see that both NF-ResNets and SkipInit with Scaled Weight Standardization can match the performance of batch normalization on both ResNet50 and ResNet200 when the batch size is not too large (less than 4096). However, SkipInit, both with and without Scaled Weight Standardization, can be somewhat unstable (indicated by $^\star$ in Table \ref{table:resnet_block_ablations}), while NF-ResNets were more stable in our experiments.

Additionally, we note that while the differences between the different methods are small for ResNet50 (particularly when the batch size is not too large), they are bigger on the deeper ResNet200 model. We see that using either $\alpha$-scaling (modification (3)) or SkipInit (modification (4)) can help train the deeper ResNet200, and using both together provides both the most stable performance for NF-ResNets, while matching the performance of batch normalized networks.
